# Supplementary material for: Scaled tree fractals do not strictly self-assemble
Source: arXiv:1411.3044 source file (2014-11-12)
Supplement: Supplementary file 1 [file appendix.tex]

\newpage
\noindent{\bf Appendix}

\begin{definition}
If $G$ is the generator of any $g$-discrete self-similar
fractal, then the \emph{interior} of $G$ is $G \cap (\N_{g-1}\times \N_{g-1})$.
\end{definition}

\begin{comment}
\begin{definition}
Let $S$ be any finite subset of $\Z^2$. A \emph{double-bridge point}
of $S$ is a point of $S$ that belongs to both an h-bridge and a
v-bridge of $S$.
\end{definition}
\end{comment}

\setcounter{theorem}{0}
\setcounter{lemma}{0}

\begin{lemma}
\label{lem:app-north-free-point}
Let $G$ be any finite subset of $\N^2$ that has at least one connected
h-bridge. If $G$ contains a connected component $C \subset G$ such
that $C \cap (\N \times \{t_G\}) \ne \emptyset$ and $C \cap (\{l_G\}
\times \N) = \emptyset$, then there exists a point $\vec{x}_N \in G
\backslash C$ such that $\vec{x}_N \not \in \N \times \{t_G\}$ and 
$\vec{x}_N$ is north-free in $G$.
\end{lemma}

\begin{proof}
Let $h$ be a connected h-bridge in $G$ and let $\pi$ be a path in $G$
connecting the two points in $h$. Since $\pi$ connects the leftmost
and rightmost columns of $G$ and $C$ does not contain any point in the
leftmost column of $G$, $C \cap \pi = \emptyset$. Since $C$ is a
connected component that extends vertically from row $t_C = t_G$ down
to row $b_C$ and $C \cap \pi = \emptyset$, $\pi$ must go around (and
below) $C$. Furthermore, no point in $C$ is adjacent to any point in
$\pi$. Let $\vec{p}$ denote a bottommost point $(x,b_C)$ in $C$, with
$l_G < x \leq r_G$. Let $\vec{q}$ denote the topmost point $(x,y)$ in
$\pi \cap (\{x\}\times \mathbb{N}_{b_C})$. Note that $\vec{p}$ and
$\vec{q}$ are in the same column, $\vec{p}$ is above $\vec{q}$, and
$G$ contains no points between $\vec{p}$ and $\vec{q}$ in that
column. Since $\vec{p}$ is not adjacent to $\vec{q}$, $y <
b_C-1$. Therefore, $\vec{q}$ is north-free in $G$. Since $\vec{q} \in \pi
\subset G$ and $\vec{q} \not\in C$, $\vec{q} \in G\backslash
C$. Furthermore, since $\vec{q}=(x,y)$ and $y < b_C -1 < b_C \leq t_C
= t_G$, $\vec{q} \not \in \mathbb{N} \times \{t_G\}$. In conclusion,
$\vec{q}$ exists and is a candidate for the role of $x_N$.  \qed
\end{proof}

\begin{lemma}
\label{lem:app-north-east-free-point}
Let $G$ be any finite subset of $\N^2$ that has at least one connected
v-bridge. If $G$ contains a connected component $C \subset G$ such
that $C \cap (\{r_G\} \times \N ) \ne \emptyset$, $C \cap (\N \times
\{t_G\}) \ne \emptyset$ and $C \cap (\N \times \{b_G\}) = \emptyset$,
then there exists a point $\vec{x}_{NE} \in G \backslash C$ such that
$\vec{x}_{NE} \in \N \times \{t_G\}$, $\vec{x}_{NE} \not \in \{r_G\} \times \N$, and $\vec{x}_{NE}$ is east-free in $G$.
\end{lemma}

\begin{proof}
Let $v$ be a connected v-bridge in $G$ and let $\pi$ be a path in $G$
connecting the two points in $v$. Let $\pi_{t}$ denote $\pi \cap (\N
\times \{t_G\})$. Since $\pi_t$ cannot be empty, the point $\vec{p} =
(r_{\pi_t},t_G)$ must exist. Similarly, let $C_{t}$ denote $C \cap (\N
\times \{t_G\})$. Since $C_t$ cannot be empty, the point $\vec{q} =
(l_{C_t},t_G)$ must exist.

Since $\pi$ connects the topmost and bottommost rows of $G$ and $C$
does not contain any point in the bottommost row of $G$, $C \cap \pi =
\emptyset$. This, together with the fact that $C$ contains a path from
the topmost row to the rightmost column of $G$ (that is, $C$ ``cuts off'' the
subset of $G$ that lies to the north-east of $C$ from the rest of
$G$), implies that all of the points in $\pi_{t}$ must appear to the
left of all the points in $C_{t}$, namely $r_{\pi_{t}} <
l_{C_{t}}$. In fact, since $\pi$ and $C$ cannot be connected,
$\vec{p}$ and $\vec{q}$ cannot be adjacent, i.e., $r_{\pi_{t}} <
l_{C_{t}}-1$. Therefore, $\vec{p}$ and $\vec{q}$ are both in the
topmost row of $G$ (thus $\vec{p} \in \N \times \{t_G\}$), $\vec{p}$ is
to the left of $\vec{q}$ (thus $\vec{p} \not \in \{r_G\} \times
\mathbb{N}$), and $G$ does not contain any points in the topmost row
between the non-adjacent points $\vec{p}$ and $\vec{q}$ (thus
$\vec{p}$ is east-free in $G$). In conclusion, $\vec{p} \in \pi \subseteq
G \backslash C$ is a candidate for the role of $\vec{x}_{NE}$.\qed
\end{proof}

\begin{lemma}
\label{lem:app-east-free-point}
Let $G$ be any finite subset of $\N^2$ that has at least one connected
v-bridge. If $G$ contains a connected component $C \subset G$ such
that $C \cap (\{r_G\} \times \N ) \ne \emptyset$, and $C \cap
(\N \times \{b_G\}) = \emptyset$, then there exists a point
$\vec{x}_{E} \in G \backslash C$ such that
$\vec{x}_{E} \not \in \{r_G\} \times \mathbb{N}$ and $\vec{x}_{E}$ is
east-free in $G$.
\end{lemma}

\begin{proof}
Let $v$ be a connected v-bridge in $G$ and let $\pi$ be a path in $G$
connecting the two points in $v$. Since $\pi$ connects the topmost and
bottommost rows of $G$ and $C$ does not contain any point in the
bottommost row of $G$, $C \cap \pi = \emptyset$. Since $C$ is a
connected component that extends horizontally from column $l_C$ to
column $r_C=r_G$ and $C \cap \pi = \emptyset$, $\pi$ must go around
(and to the left of) $C$. Furthermore, no point in $C$ is adjacent to
any point in $\pi$.  Let $\vec{p}$ denote a leftmost point $(l_C,y)$
in $C$, with $b_G < y \leq t_G$. Let $\vec{q}$ denote the rightmost
point $(x,y)$ in $\pi \cap (\N_{l_C}\times \{y\})$. Note that
$\vec{p}$ and $\vec{q}$ are in the same row, $\vec{q}$ is to the left of
$\vec{p}$, and $G$ contains no points between $\vec{p}$ and $\vec{q}$
in that row. Since $\vec{p}$ is not adjacent to $\vec{q}$, $x <
l_C-1$. Therefore, $\vec{q}$ is east-free in $G$. Since $\vec{q} \in \pi
\subset G$ and $\vec{q} \not\in C$, $\vec{q} \in G\backslash
C$. Furthermore, since $\vec{q}=(x,y)$ and $x < l_C -1 < l_C \leq r_C
= r_G$, $\vec{q} \not \in \{r_G\}\times \N$. In conclusion,
$\vec{q}$ exists and is a candidate for the role of $x_E$.  \qed
\end{proof}

\begin{theorem}
$\mathbf{T} = \bigcup_{i=0}^{\infty}{T_i}$ is a $g$-discrete self-similar tree fractal, for some $g > 1$, with generator $G$ if and only if \\
\hspace*{1cm}a. $G$ is a tree, and\\
\hspace*{1cm}b. $nhb_G = nvb_G =1$
\end{theorem}

\begin{proof}
\verb+[+still needs to be checked, together with the proofs of all supporting lemmas\verb+]+
\end{proof}

\begin{lemma}[Closed Window Movie Lemma]\label{lem:app-wml}
Let $\vec{\alpha}~=~(\alpha_i~|~0\leq~i<~l)$, with $l \in \mathbb{Z}^+
\cup \{\infty\}$, be an assembly sequence in some TAS $\mathcal{T}$
with result $\alpha$. Let $w$ be a closed window that partitions
$\alpha$ into $\alpha_I$ and $\alpha_O$, and $w'$ be a closed window
that partitions $\alpha$ into $\alpha_I'$ and $\alpha_O'$.  If
$\mathcal{B}(M_{\vec{\alpha},w}) + \vec{c} =
\mathcal{B}(M_{\vec{\alpha},w'})$ for some $\vec{c}\neq(0,0)$ and
the window $w+\vec{c}$ is enclosed in $w'$, then the assembly $\alpha'_O \cup (\alpha_I + \vec{c})$ is
in $\mathcal{A[\mathcal{T}]}$.
\end{lemma}

\begin{proof}
\verb+[+included in Section 2.3 of the paper\verb+]+
\end{proof}

\begin{comment}
\begin{lemma}
\label{lem:app-free-point-with-orthogonal-pier}
Let $G$ be the generator of any $g$-discrete self-similar fractal. If
$G$ contains an east-pointing pier that is the
northmost point in a v-bridge of $G$, then $G$ contains an interior
north-free point.
\end{lemma}

\begin{proof}
Let $(p,g-1)$ be the pier considered in the hypothesis of the lemma.
In this case, $(p,0) \in G$ (since $(p,g-1)$ belongs to a v-bridge)
and $(p,g-2) \not\in G$ (since $(p,g-1)$ is an east-pointing pier;
note that in this case, $g$ must be greater than 2; otherwise,
$(p,g-1)$ could not be an east-pointing pier). Therefore, there must
exist at least one point in $G \cap (\{p\} \times \N_{g-2})$, say
$(p,y)$, with $0 \leq y < g-2$, that is north-free. If $p<g-1$, then
$(p,y)$ is an interior north-free point of $G$. If $p=g-1$, then we
know that $(0,g-1) \not\in G$ (otherwise $G$ would contain two
h-bridges and two v-bridges, which would contradict
Theorem~\ref{thm:tree-fractal}).  Since $(0,0)\in G$, $G \cap
(\{0\} \times \N_{g-1})\neq \emptyset$. Let $(0,y)$ denote the topmost
point in $G \cap (\{0\} \times \N_{g-1})$, with $0\leq y < g-1$. $(0,y)$
point is an interior north-free point of $G$.
\qed
\end{proof}
\end{comment}

\begin{lemma} \label{lem:app-piers}
Let $\mathbf{T}$ be any tree fractal with generator $G$. If $c \in
\mathbb{Z}^+$, then it is always possible to pick one pier $(p,q)$
and one point $(e,f)$, both in $G$, such that, for $s \in \N\,\backslash
\{0,1\}$, $W^c_s(e,f,p,q)$ encloses a configuration that is connected
to $\mathbf{T}^c$ via a single connected (horizontal or vertical) line
of glues of length $c$.
\end{lemma}

\begin{proof}
Let $\mathbf{T}$ be any tree fractal with generator $G$. Let $c \in
\mathbb{Z}^+$ and $s \in \N\,\backslash
\{0,1\}$. According to Observation~\ref{obs:piers}, $G$ must
contain at least two piers. We will pick one of these piers
carefully. Note that there are four types of piers, depending on how
many bridges they belong to. Since, by Theorem~\ref{thm:tree-fractal},
$G$ must contain exactly one h-bridge and exactly one v-bridge, the
chosen pier can belong to no more than two bridges.  A \emph{real
pier} is a pier that does not belong to any bridge in $G$. A
\emph{single-bridge pier} belongs to exactly one bridge. A
\emph{double-bridge pier} belongs to exactly two bridges. Finally, 
we will distinguish between two sub-types of single-bridge piers. If
the pier is pointing in a direction that is parallel to the direction
of the bridge (i.e., if the pier points north or south and belongs to
a v-bridge, or the pier points east or west and belongs to an
h-bridge), the pier is a \emph{parallel single-bridge pier}. If the
pier is pointing in a direction that is orthogonal to the direction of
the bridge (i.e., if the pier points north or south and belongs to an
h-bridge, or the pier points east or west and belongs to a v-bridge),
the pier is an \emph{orthogonal single-bridge pier}.

First, we observe that it is always possible to choose a pier in $G$
that is not a double-bridge pier. Indeed, if one of the piers in $G$
is a double-bridge pier, then none of the other piers in $G$ can
be double-bridge piers. Otherwise, the presence of two distinct
double-bridge points in $G$ would imply that
$\{(0,0),(0,g-1),(g-1,0),(g-1,g-1)\} \subset G$. $G$ would thus contain
two h-bridges and two v-bridges, which would contradict
Theorem~\ref{thm:tree-fractal}. Therefore, we can always choose either
a real pier or a single-bridge pier.

Second, we observe that if $G$ contains one or more real piers, we can
simply choose one of them as $(p,q)$. In this case, we pick
$(e,f)=(p,q)$, since any window of the form $W^c_s(p,q,p,q)$, where
$(p,q)$ is a real pier in $G$, must have exactly three free
sides. Therefore, $W^c_s(p,q,p,q)$ must enclose a configuration that
is connected to $\mathbf{T}^c$ via a single line of glues of length
$c$, namely on its non-free side.

Third, if $G$ does not contain any real piers, $G$ must contain at
least one single-pier bridge. If $G$ contains at least one parallel
single-bridge pier, we choose one of them, say $(p,q)$. Without loss
of generality, assume that this pier is pointing north, that it
belongs to a v-bridge and that $q=g-1$ (a similar reasoning holds if
$q=0$, or if the pier points south, or if the pier belongs to an
h-bridge and points either west or east). Now, we must pick a point
$(e,f)$ such that any window of the form $W^c_s(e,f,p,q)$ has exactly
three free sides. We distinguish two cases.  
\begin{enumerate}
\item If $p=0$, that is, the pier is in the leftmost column of $G$, then
$(1,g-1) \not\in G$, since $(0,g-1)$ is a north-pointing
pier. Therefore, there must exist at least one point in $G \cap
(\{1\} \times \N_{g-1})$, say $(1,y)$, with $0 \leq y < g-1$, that is
north-free. In this case, we pick $(e,f)$ to be equal to $(1,y)$.
Now, consider any window $w$ of the form $W^c_s(e,f,p,q)$. The north
side of $w$ is free (since $(e,f)$ is north-free in $G$ and $f=y<g-1$),
the east side of $w$ is free (since $(1,g-1)\not\in G$), and the west
side of $w$ is free (since the facts that $(0,0)\in G$, $(0,g-1)\in G$
and $(0,g-1)$ is a single-bridge pier together imply that
$(g-1,g-1) \not\in G$). Furthermore, since $(0,g-1)$ is a
north-pointing pier, $S(0,g-1) \in G$.
\item If $p>0$, then $(p-1,g-1)\not\in G$. Therefore, there must exist 
at least one point in $G \cap (\{p-1\} \times \N_{g-1})$, say
$(p-1,y)$, with $0 \leq y < g-1$, that is north-free. In this case, we
pick $(e,f)$ to be equal to $(p-1,y)$.  Now, consider any window $w$
of the form $W^c_s(e,f,p,q)$. The north side of $w$ is free (since
$(e,f)$ is north-free in $G$ and $f=y<g-1$), the west side of $w$ is
free (because $(p-1,g-1)\not\in G$), and the east side of $w$ is free
(since, either $p<g-1$ and $(p+1,g-1)\not\in G$, or $p=g-1$, in which
case the facts that $(g-1,g-1)\in G$, $(g-1,0)\in G$ and $(g-1,g-1)$
is a single-bridge pier together imply that $(0,g-1) \not\in
G$). Furthermore, since $(p,g-1)$ is a north-pointing pier,
$S(p,g-1) \in G$. 
\end{enumerate}
Therefore, in both cases, $W^c_s(e,f,p,q)$ has exactly three free
sides and encloses a configuration that is connected
to $\mathbf{T}^c$ via a single connected horizontal line
of glues of length $c$ positioned on the south side of the window.

Finally, if $G$ does not contain any real piers nor any parallel
single-bridge piers, it must contain at least one orthogonal
single-bridge pier (since $G$ must contain at least one single-bridge
pier). We choose one of them, say $(p,q)$. Without loss of generality,
assume that this pier is pointing east, that it belongs to a v-bridge
and that $q=g-1$ (a similar reasoning holds if $q=0$, or if the pier
points west, or if the pier belongs to an h-bridge and points either
north or south). Note that, in this case, $g$ must be strictly greater
than 2, since $(p,g-1)\in G$, $(p,0)\in G$ but $(p,g-2)\not\in
G$. Now, we must pick a point $(e,f)$ such that any window of the form
$W^c_s(e,f,p,q)$ has exactly three free sides. We distinguish two
cases.
\begin{enumerate}
\item If $p<g-1$, then $(p,g-2)\not\in G$,
since $(p,g-1)$ is an east-pointing pier Therefore, there must exist
at least one point in $G \cap (\{p\} \times \N_{g-2})$, say $(p,y)$,
with $0 \leq y < g-2$, that is north-free. In this case, we pick
$(e,f)$ to be equal to $(p,y)$.  Now, consider any window $w$ of the
form $W^c_s(e,f,p,q)$. The north side of $w$ is free (since $(e,f)$ is
north-free in $G$ and $f=y<g-2<g-1$), the east side of $w$ is free
(since $p<g-1$ and $(p+1,g-1)\not\in G$), and the south side of $w$ is
free (since $(p,g-2)\not\in G$). Furthermore, since $(p,g-1)$ is an
east-pointing pier, $W(p,g-1) \in G$.
\item If $p=g-1$, that is, the pier is in the rightmost column of $G$, then
the facts that $(g-1,0) \in G$, $(g-1,g-1)\in G$ and $(g-1,g-1)$ is a
single-bridge pier together imply that $(0,g-1)\not\in G$. This,
together with the fact that $(0,0)\in G$, implies that there must
exist at least one point in $G \cap (\{0\} \times \N_{g-1})$, say
$(0,y)$, with $0 \leq y < g-1$, that is north-free. In this case, we
pick $(e,f)$ to be equal to $(0,y)$. Now, consider any window $w$ of
the form $W^c_s(e,f,p,q)$. The north side of $w$ is free (since
$(e,f)$ is north-free in $G$ and $f=y<g-1$), the east side of $w$ is free
(since $(0,g-1)\not\in G$), and the south side of $w$ is free (since
$(p,g-2)\not\in G$). Furthermore, since
$(g-1,g-1)$ is an east-pointing pier, $W(g-1,g-1) \in G$. 
\end{enumerate}
Therefore, in both cases, $W^c_s(e,f,p,q)$ has exactly three free
sides and encloses a configuration that is connected
to $\mathbf{T}^c$ via a single connected horizontal line
of glues of length $c$ positioned on the west side of the window.
\qed
\end{proof}

\begin{lemma}\label{lem:app-enclosure2}
Let $i, j, c \in \mathbb{Z}^+$, with $i<j$, $e, f,p,q \in
\mathbb{N}_g$, and $x,y \in \mathbb{N}$. Let $m =
c(g^{j-2}-g^{i-2})$. If $x\leq m$ and $y\leq m$, then the window
$W^c_i(e,f,p,q) +\vec{t}^c_{i\rightarrow j}(e,f,p,q)+(x,y)$ is
enclosed in the window $W^c_j(e,f,p,q)$.
\end{lemma}

\begin{proof}
Let $W$ and $w$ denote $W^c_j(e,f,p,q)$ and
$W^c_i(e,f,p,q)+\vec{t}^c_{i\rightarrow j}(e,f,p,q)$,
respectively. Since $W$ and $w$ are square windows that have the same
southwest corner and whose respective sizes are $cg^{j-2}$ and
$cg^{i-2}$, $W$ encloses $w$. The eastern side of $w + (x,0)$ still
lies within $W$, because the maximum value of $x$ is equal to the
difference between the size of $W$ and the size of $w$. The same
reasoning applies to a northward translation of $w$ by $(0,y)$. In
conclusion, $w+(x,y)$ must be enclosed in $W$, as long as neither $x$
nor $y$ exceeds $m$.\qed
\end{proof}
